# Supplementary material for: On the Effectiveness of Automated Metrics for Text Generation Systems
Source: arXiv:2210.13025 source file (2022-10-24)
Supplement: Supplementary file 1 [file stb_pairwise_additional.tex]

\begin{tabular}{ c | c c c c c c }
     & BL   & LiC   & KV   & HF   & BR   & S2S   \\ \hline
    
        BL  & -  & 0.08 (0.999)  & 0.13 (1.000)  & 0.20 (1.000)  & 0.31 (1.000)  & 0.33 (1.000)  \\
    
        LiC  & -0.08 (0.001)  & -  & 0.06 (0.991)  & 0.12 (1.000)  & 0.23 (1.000)  & 0.25 (1.000)  \\
    
        KV  & -0.13 (0.000)  & -0.06 (0.009)  & -  & 0.07 (0.999)  & 0.17 (1.000)  & 0.20 (1.000)  \\
    
        HF  & -0.20 (0.000)  & -0.12 (0.000)  & -0.07 (0.001)  & -  & 0.11 (1.000)  & 0.13 (1.000)  \\
    
        BR  & -0.31 (0.000)  & -0.23 (0.000)  & -0.17 (0.000)  & -0.11 (0.000)  & -  & 0.02 (0.965)  \\
    
        S2S  & -0.33 (0.000)  & -0.25 (0.000)  & -0.20 (0.000)  & -0.13 (0.000)  & -0.02 (0.032)  & -  \\
    
\end{tabular}
